# Supplementary material for: Deep Spectral Clustering via Joint Spectral Embedding and Kmeans
Source: arXiv:2412.11080 source file (2024-12-15)
Supplement: Supplementary file 1 [file sec_appendix.tex]

\newpage
\appendix
\section{Mathematical Proof for the Greedy Optimization Strategy}
Here a mathematical proof for the effectiveness of the greedy optimization strategy in Equation \ref{eqn:finetune} is provided.
Note that the cluster structures
of Kmeans can be measured by entropy. The lower the entropy of data, the higher the cluster structures it contains. 
Therefore, the goal is to demonstrate that the entropy of target random vector $\mathbf{y}$ is lower than that of random vector $\mathbf{t}$.
For conciseness, random vector $\mathbf{t}=\left[{t}^1,\cdots,{t}^d\right]$ is denoted by $\mathbf{x}=\left[{x}_1,\cdots,{x}_d\right]$. Similarly, target random vector $\mathbf{y}=\left[{t}^1,\cdots,{t}^{d-1},y\right]$ is denoted by $\mathbf{y}=\left[{x}_1,\cdots,{x}_{d-1},y\right]$, where random variable $y$ with domain in Equation \ref{eq_y}.
Supposing all random variables ${x}_1,\cdots,{x}_d$ are mutually independent.

Let us start with the case of $d=2$, where $\mathbf{x}=\left[{x}_1,{x}_2\right]$ and  $\mathbf{y}=\left[{x}_1,{y}\right]$.
According to the definition of  joint entropy, $h(\mathbf{x})$ can be written as follows:
\begin{equation}
		h(\mathbf{x})=h({x}_1,{x}_2)=h({x}_1)+h({x}_2\mid {x}_1)
\end{equation}

Since ${x}_1$ and ${x}_2$ are independent, $h(\mathbf{x})$ can be further written as follows:
\begin{equation}
	\begin{aligned}
		h(\mathbf{x})=h({x}_1)+h({x}_2)
	\end{aligned}
\end{equation}

Similarly, the entropy of $\mathbf{y}$ is:
\begin{equation}
	\label{eq_hy}
	\begin{aligned}
		h(\mathbf{y})=h({y})+h({x}_1\mid{y})
	\end{aligned}
\end{equation}

Considering the monotonicity property of conditional entropy $h({x}_1\mid{y}) \le h({x}_1)$, the difference between $h(\mathbf{x})$ and $h(\mathbf{y})$ can be written as:
\begin{equation}
	\label{eq_hx_hy}
	\begin{aligned}
		h(\mathbf{x})-h(\mathbf{y}) \ge h({x}_2)-h({y})
	\end{aligned}
\end{equation}

Now our goal is to demonstrate $h({x}_2)-h({y}) > 0$. In the rest of this section, ${x}_2$ is denoted by ${x}$ for conciseness. 
Since ${x}$ is a continuous random variable and its probability density function, of course, is unknown, ${x}$ needs to be quantized for calculating entropy. 
${x}_\Delta$ is defined as the uniformly quantized version of ${x}$ with quantization step-size $\Delta$:
\begin{equation}
	x_{\Delta}=i    \qquad  \text{if} \quad  x \in[i \Delta,(i+1) \Delta)
\end{equation}
i.e., the domain of $x$ is divided into many intervals. 
All $x$ in the same interval have the same $x_{\Delta}$, while $x$ in different intervals have different $x_{\Delta}$.
And without loss of generality, supposing there are $m$ non-empty intervals and the $i$-th non-empty interval has $p_i$ samples, where $1 \le i \le m, 1\le p_i \le n$.
An empty interval having no sample is discarded, whose entropy is zero.
We have the following:
\begin{equation}
	\label{eq_pi_limit}
	{p_1}+\cdots+{p_m}=n
\end{equation}

Similarly, ${y}$ is quantized  with the same quantization step-size $\Delta$. According to Equation \ref{eq_y}, the size of the support of random variable ${y}$ is $k$.
Therefore, there are up to $k$ non-empty intervals. 
There is no harm in supposing that only $k$ intervals happen to be non-empty because the entropy of an empty interval is zero. 
The number of samples in the $i$-th non-empty interval is denoted by $n_i$, where $1 \le i \le k, 1 \le n_i \le n$. Also, we have the following:
\begin{equation}
	\label{eq_ni_limit}
	{n_1}+\cdots+{n_k}=n
\end{equation}

According to the Rényi theorem \cite{renyi1959dimension}, when quantization step-size  $\Delta$ is small the relation between $h({x})$ and the quantized $H({x}_\Delta)$ is:
\begin{equation}
	\label{hx_hxdelta}
	h({x})=H({x}_{\Delta})+\log \Delta
\end{equation}

With the definition of entropy, $H({x}_{\Delta})$ is defined as:
\begin{equation}
	\label{eq_Hx_define}
	\begin{aligned}
		H({x}_{\Delta}) &=  - \sum\limits_x {p(x_{\Delta})\log p(x_{\Delta})}  \hfill \\
		&=  - (\frac{{{p_1}}}{n}\log \frac{{{p_1}}}{n} +  \cdots  + \frac{{{p_m}}}{n}\log \frac{{{p_m}}}{n}) \hfill \\
		&= \log n - \sum\limits_{i = 1}^m {\frac{{{p_i}}}{n}\log {p_i}}  \hfill \\ 
	\end{aligned}
\end{equation}

Similarly, for ${y}$ we have:
\begin{equation}
	\label{hy_hydelta}
	h({y})=H({y}_{\Delta})+\log \Delta
\end{equation}
\begin{equation}
	\label{eq_Hy_define}
	\begin{aligned}
		H({y}_{\Delta}) = \log n - \sum\limits_{i = 1}^k {\frac{{{n_i}}}{n}\log {n_i}} 
	\end{aligned}
\end{equation}

Combined with Equations \ref{hx_hxdelta}--\ref{eq_Hy_define}, the difference between $h({x})$ and $h({y})$ can be written as:
\begin{equation}
	\label{eq_hx_hy_obj}
	\begin{aligned}
		h({x}) - h({y}) = \sum\limits_{i = 1}^k {\frac{{{n_i}}}{n}\log {n_i}}  - \sum\limits_{i = 1}^m {\frac{{{p_i}}}{n}\log {p_i}}
	\end{aligned}
\end{equation}

Recall that our goal is to demonstrate $h({x})-h({y}) > 0$.
To this end, let us consider Equation \ref{eq_hx_hy_obj} as a constrained optimization problem. Note that it subjects to equality constraints of Equations \ref{eq_pi_limit}--\ref{eq_ni_limit}. Given a dataset, $n$ is a known constant. Therefore, the optimization problem can be formulated to:
\begin{equation}
	\label{eq_j}
	\begin{aligned}
		\mathcal{J}(n_{1}, \cdots,&n_{k},~ p_{1},\cdots,p_{m}) =n\left(h\left({x}\right)-h\left({y}\right)\right) \\
		&=\sum_{i=1}^{k} n_{i} \log n_{i}-\sum_{i=1}^{m} p_{i} \log p_{i} \\
		& \text {s.t. }\left\{\begin{array}{c}
			p_{1}+\cdots+p_{m}=n \\
			n_{1}+\cdots+n_{k}=n
		\end{array}\right.
	\end{aligned}
\end{equation}

Applying the Lagrange multiplier method yields:
\begin{equation}
	\begin{aligned}
		\mathcal{F}&(n_{1}, \cdots, p_{m}, \lambda_{1}, \lambda_{2})=\sum_{i=1}^{k} n_{i} \log n_{i}-\sum_{i=1}^{m} p_{i} \log p_{i}\\
		&+\lambda_{1}\left(n-n_{1}-\cdots-n_{k}\right)+\lambda_{2}\left(n-p_{1}-\cdots-p_{m}\right)
	\end{aligned}
\end{equation}
from which the gradient can be calculated and set to zero:
\begin{equation}
	\left\{\begin{array}{c}
		\frac{\partial \mathcal{F}}{\partial n_{1}}=\log n_{1}+\frac{1}{\ln 2}-\lambda_{1}=0 \\
		\vdots \\
		\frac{\partial \mathcal{F}}{\partial p_{m}}=\log p_{m}+\frac{1}{\ln 2}-\lambda_{2}=0 \\
		\frac{\partial \mathcal{F}}{\partial \lambda_{1}}=n-n_{1}-\cdots-n_{k}=0 \\
		\frac{\partial \mathcal{F}}{\partial \lambda_{2}}=n-p_{1}-\cdots-p_{m}=0
	\end{array}\right.
\end{equation}

Solving the above equations yields:
\begin{equation}
	\label{eq_criticalpoint}
	\left\{\begin{array}{l}
		n_{i}=\frac{n}{k}, i=1, \cdots, k \\
		p_{i}=\frac{n}{m}, i=1, \cdots, m
	\end{array}\right.
\end{equation}
which implies that the critical
point in the above equations will yield an extremum for the function $\mathcal{J}$. 
To determine the maximum or the minimum extremum, the second partial derivatives are calculated:
\begin{equation}
	\left\{ {\begin{array}{*{20}{c}}
			{\frac{{{\partial ^2}\mathcal{F}}}{{\partial n_1^2}} = \frac{1}{{{n_1}\ln 2}} > 0} \\ 
			\vdots  \\ 
			{\frac{{{\partial ^2}\mathcal{F}}}{{\partial p_m^2}} = \frac{1}{{{p_m}\ln 2}} > 0} 
	\end{array}} \right.
\end{equation}

With the above equations, we know that the extremum is a minimum. 
Substituting critical point in Equation \ref{eq_criticalpoint} into function $\mathcal{J}$ in Equation \ref{eq_j}, the minimum is:
\begin{equation}
	\mathcal{J}_{\text{extremum}}=n\log \frac{m}{k}
\end{equation}

For real-world datasets, the number of unique entries of $x$ is much large than $k$, i.e., $m\gg k$. Therefore, we have:
\begin{equation}
	h({x})-h\left({y}\right)=\frac{1}{n}\mathcal{J}\ge  \log \frac{m}{k} >0
\end{equation}

Finally, according to Equation (\ref{eq_hx_hy}), we have:
\begin{equation}
	h(\mathbf{x})-h(\mathbf{y}) >0	
\end{equation}   

Here we demonstrate that the entropy of target $\mathbf{y}$ is lower than that of $\mathbf{x}$, which indicates $\mathbf{Y}$ contains more cluster structures than $\mathbf{T}$. Therefore, our optimization method in Equation \ref{eqn:finetune} is effective.

Now we generalize this conclusion to the general case without requiring $d=2$. Due to all random variables $\mathbf{x}_i$ are mutually independent, $h(\mathbf{x})$ is equal to:
\begin{equation}
		h(\mathbf{x})= h({{{x}_1}, \cdots ,{{x}_d}})=\sum_{i=1}^d h({x}_i)
\end{equation}

With the chain rule $h(\mathbf{y})$ is:
\begin{equation}
	\begin{aligned}
		h(\mathbf{y})&=h\left({x}_{1}, \cdots, {x}_{d-1}, {y}\right) =h({y})+h({x}_1 \mid {y})\\
		&+h({x}_2 \mid {y}, {x}_1)+\cdots+h({x}_{d-1} \mid {y},\cdots, {x}_{d-2})
	\end{aligned}
\end{equation}

Then $h(\mathbf{x})-h(\mathbf{y})$ can be written as:
\begin{equation}
	\begin{aligned}
		h(\mathbf{x})-&h(\mathbf{y}) =h\left({x}_{d}\right)-h({y})+\left[h\left({x}_1\right)-h\left({x}_{1} \mid {y}\right)\right]\\
		&+\cdots+\left[h\left({x}_{d-1}\right)-h\left({x}_{d-1} \mid {y}, \cdots, {x}_{d-2}\right)\right]
	\end{aligned}
\end{equation}

Applying the monotonicity property of conditional entropy, the above equation can be  further rewritten as:
\begin{equation}
	h(\mathbf{x})-h(\mathbf{y})\ge h({x}_d)-h({y})
\end{equation}

This comes back to Equation (\ref{eq_hx_hy}) and here we won't repeat that again.
